# Supplementary material for: The Bernstein-von Mises theorem for Semiparametric Mixtures
Source: arXiv:2412.00219 source file (2024-11-29)
Supplement: Supplementary file 1 [file Supplements.tex]

\section{General supplementary material}
\TODO{check if needs to be removed}
\begin{lem}\label{lem:ErrorsInVarsPriorMassBound}
    Suppose that all assumptions of \Cref{lem:ErrorsInVarsPriorMassEps} are satisfied.
    Then
    \[
        \frac{e^{- c\sqrt{n} \log n}}{ \pi_t \otimes \textrm{DP}_t (B_{n,2} (p_{\theta, F}; p_{\theta_0, F_0}, \epsilon_n))} = o(e^{-2n \epsilon_n^2})
    \]
\end{lem}

\begin{proof}
    Pick $\epsilon_n = n^{-\alpha}$ for $a = \frac{1}{2}$.
    By \Cref{lem:ErrorsInVarsPriorMassEps} we know that
    \begin{align*}
        \pi_t \otimes \textrm{DP}_t(B_{n,2} (p_{\theta, F}; p_{\theta_0, F_0}, \epsilon_n)) &\leq= \pi \otimes \textrm{DP}_t( \textrm{KL} + V_2 \left( p_{\theta, F}; p_{\theta_0, F_0} \right) \leq \epsilon_n^2 )\\
            &\geq e^{-C \epsilon_n^{-\frac{1}{( 1 + \xi)}} \log( \epsilon_n^{-1})} \\
            &= e^{ - C' n^{\frac{\alpha}{(1 + \xi)}} \log n}
    \end{align*}
    Hence we want to show that
    \[
        e^{C n^{ \frac{\alpha}{2( 1 + \xi)}} \log n} e^{- c \sqrt{n} \log n} e^{2 n^{1 - 2 \alpha}} = o(1)
    \]
    It suffices to show that $\sqrt{n} \log(n)$ dominates both other terms.
    $n \epsilon_n^2 = n^{1 - 2 \alpha}$ is much smaller than $n^{1/2}\log(n)$ as soon as $\alpha \geq \frac{1}{4}$.
    For the choice $\alpha = \frac{1}{2}$ we get $n \epsilon_n^2 = 1$, and hence this term does not contribute.
    Now we need to show that $\sqrt{n} \log n$ also dominates $n^{\frac{\alpha}{(1 + \xi)}} \log (n)$.
    It suffices to show that $\frac{\alpha}{(1 + \xi)} < \frac{1}{2}$.
    This holds true as soon as $\alpha < \frac{1 + \xi}{2}$, which is true since $\xi > 0$.
\end{proof}
